# Supplementary material for: Pairwise likelihood estimation of latent autoregressive count models
Source: arXiv:1805.10865 source file (2020-06-22)
Supplement: Supplementary file 1 [file pedeli-varin-supplement-revision-v6.pdf]

# Supplementary materials of 'Pairwise likelihood estimation of latent autoregressive count models'

Xanthi Pedeli and Cristiano Varin

February 25, 2020

These supplementary materials consist of two sections. The first section describes how to use the R package `lacm` for reproduction of the real data analyses contained in Section 5 of the paper. The second section consists of a series of plots related to simulation study described in Section 4 of the paper.

## 1 Reproduction of results

### Invasive Meningitis in Greece

Read the invasive meningitis Greek data[1]:

```
meningo.gr <- read.csv("ECDC_meningo_gr.csv")
```

Visualize the series:

```
plot(ts(meningo.gr$cases, start = c(1999, 1), freq = 12), ylab = "Cases", xlab ="")
```

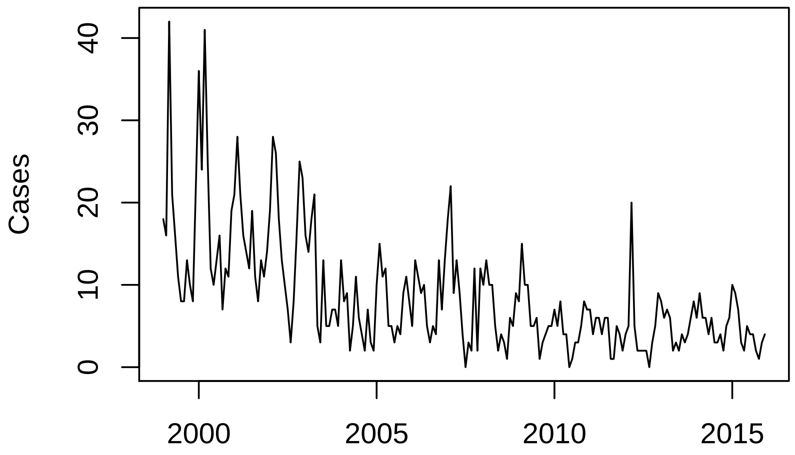


[1]The Greek and the Italian invasive meningitis data were obtained from the European Center of Disease Control (ECDC) Surveillance Atlas (`https://ecdc.europa.eu/en/surveillance-atlas-infectious-diseases`).

Build trend and annual seasonality terms:

```
meningo.gr$sin.term <- sin(2 * pi * meningo.gr$time / 12)
meningo.gr$cos.term <- cos(2 * pi * meningo.gr$time / 12)
## scaled trend
meningo.gr$trend <- meningo.gr$time / nrow(meningo.gr)
```

Fit a standard Poisson regression model and obtain the Pearson residuals:

```
mod0.gr <- glm(cases ~ trend + sin.term + cos.term, data = meningo.gr,
        family = poisson)
res0.gr <- residuals(mod0.gr,  type = "pearson")
```

Plot the sample partial autocorrelation function of the Pearson residuals to select the order $d$ of the pairwise likelihood:

```
pacf(res0.gr, main =" ")
```

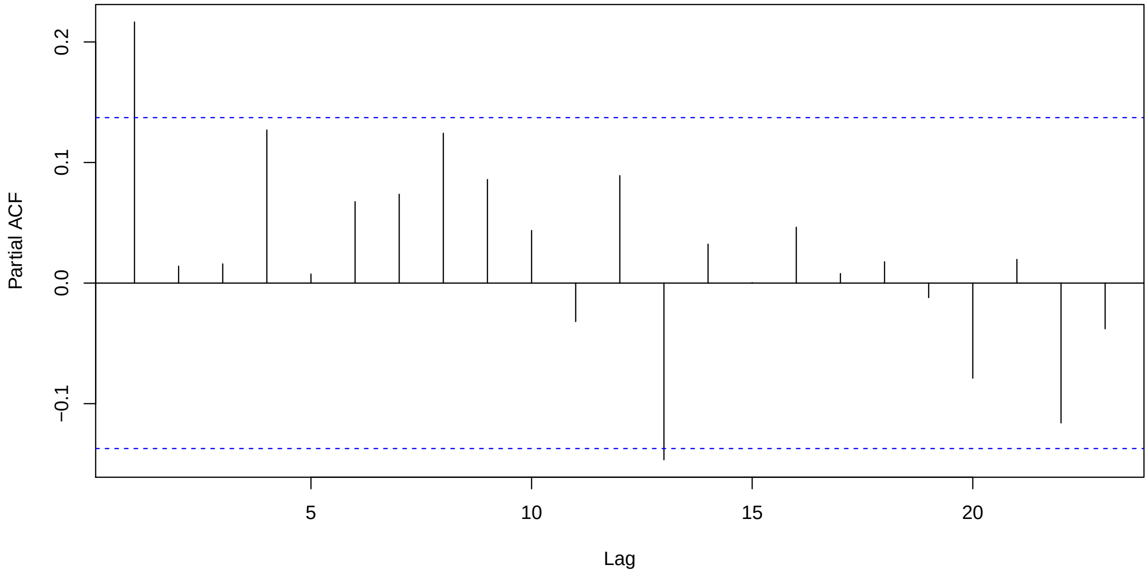


The plot suggests the presence of non-spurious correlation between pairs of observation separated by one lag. We start with a preliminary fit of the autoregressive count model using option `fit = FALSE` in `lacm`:

```
fit.gr.start <-  lacm(cases ~ trend + sin.term + cos.term, data = meningo.gr,
             d = 1, fit = FALSE)
```

Below, we calculate preliminary estimates of the dispersion indices which indicate that a low number of quadrature nodes is sufficient for approximation of the bivariate integrals of the pairwise likelihood:

```
## preliminary estimation of dispersion indices
tau2 <- fit.gr.start$start.theta[6]
eta <- fit.gr.start$X %*% fit.gr.start$start.theta[1:4]
```

```
Di <- exp(eta + tau2 / 2) * (exp(tau2) - 1)
summary(Di)

##        V1
## Min.   :0.1408
## 1st Qu.:0.3411
## Median :0.5437
## Mean   :0.6575
## 3rd Qu.:0.8459
## Max.   :2.1344
```

Accordingly, we fit the latent autoregressive count model with the pairwise likelihood of order one with trapezoidal weights approximated with Gauss-Hermite quadrature using five nodes per dimension:

```
## load the lacm library
library(lacm)
pfit5.gr <- lacm(cases ~ trend + sin.term + cos.term, data = meningo.gr,
        d = 1, kernel.type = "Trapezoidal", gh.num = 5)
print(summary(pfit5.gr), digits = 2)

##
## Call:
## lacm(formula = cases ~ trend + sin.term + cos.term, data = meningo.gr,
##    d = 1, kernel.type = "Trapezoidal", gh.num = 5)
##
## Pairwise likelihood order: 1
##
## Coefficients:
##             Estimate Std. Error z value Pr(>|z|)
## (Intercept)    2.793      0.111    25.1   <2e-16 ***
## trend         -1.684      0.222    -7.6    3e-14 ***
## sin.term       0.463      0.037    12.4   <2e-16 ***
## cos.term       0.282      0.044     6.4    2e-10 ***
## phi            0.506      0.167     3.0    0.002 **
## tau2           0.071      0.019     3.8    2e-04 ***
## ---
## Signif. codes:  0 `***' 0.001 `**' 0.01 `*' 0.05 `.' 0.1 ` ' 1
##
## Log pairwise likelihood: -1041.2,  CLIC: 2117
```

Refit with ten quadrature nodes per dimension:

```
pfit10.gr <- lacm(cases ~ trend + sin.term + cos.term, data = meningo.gr,
          d = 1, kernel.type = "Trapezoidal", gh.num = 10)
print(summary(pfit10.gr), digits = 2)

##
```

```
## Call:
## lacm(formula = cases ~ trend + sin.term + cos.term, data = meningo.gr,
##    d = 1, kernel.type = "Trapezoidal", gh.num = 10)
##
## Pairwise likelihood order: 1
##
## Coefficients:
##             Estimate Std. Error z value Pr(>|z|)
## (Intercept)    2.789      0.113    24.6   <2e-16 ***
## trend         -1.675      0.224    -7.5    8e-14 ***
## sin.term       0.462      0.037    12.5   <2e-16 ***
## cos.term       0.283      0.044     6.4    2e-10 ***
## phi            0.519      0.166     3.1    0.002 **
## tau2           0.070      0.019     3.8    2e-04 ***
## ---
## Signif. codes:  0 `***' 0.001 `**' 0.01 `*' 0.05 `.' 0.1 ` ' 1
##
## Log pairwise likelihood: -1041.3,  CLIC: 2117
```

Finally with twenty quadrature nodes per dimension:

```
pfit20.gr <- lacm(cases ~ trend + sin.term + cos.term, data = meningo.gr,
          d = 1, kernel.type = "Trapezoidal", gh.num = 20))
print(summary(pfit20.gr), digits = 2)

##
## Call:
## lacm(formula = cases ~ trend + sin.term + cos.term, data = meningo.gr,
##     d = 1, kernel.type = "Trapezoidal", gh.num = 20)
##
## Pairwise likelihood order: 1
##
## Coefficients:
##             Estimate Std. Error z value Pr(>|z|)
## (Intercept)    2.789      0.113    24.6   <2e-16 ***
## trend         -1.675      0.243    -7.5    8e-14 ***
## sin.term       0.461      0.037    12.5   <2e-16 ***
## cos.term       0.283      0.044     6.4    2e-10 ***
## phi            0.518      0.166     3.1    0.002 **
## tau2           0.070      0.019     3.8    2e-04 ***
## ---
## Signif. codes:  0 `***' 0.001 `**' 0.01 `*' 0.05 `.' 0.1 ` ' 1
##
## Log pairwise likelihood: -1041.3,  CLIC: 2117
```

Gauss-Hermite quadrature with $5 \times 5$, $10 \times 10$ and $20 \times 20$ nodes give the same estimates and standard errors up to two decimal digits. For the rest of the analysis we base ourselves on the model with $10 \times 10$ quadrature nodes.

Comparison with the reduced model without serial correlation ($\phi = 0$):

```
## refit the model fixing phi = 0
pfit10.gr.nophi <- update(formula (= cases ~ trend + sin.term + cos.term,
       data = meningo.gr, fixed = c(NA, NA, NA, NA, 0.0, NA), d = 1,
       kernel.type = "Trapezoidal", gh.num = 10)
summary(pfit10.gr.nophi)

##
## Call:
## lacm(formula = cases ~ trend + sin.term + cos.term,
##     data = meningo.gr, fixed = c(NA, NA, NA, NA, 0, NA), d = 1,
##     kernel.type = "Trapezoidal", gh.num = 10)
##
## Pairwise likelihood order: 1
##
## Coefficients:
##             Estimate Std. Error z value Pr(>|z|)
## (Intercept)  2.79567    0.09346  29.912  < 2e-16 ***
## trend       -1.68732    0.18821  -8.965  < 2e-16 ***
## sin.term     0.46074    0.03591  12.831  < 2e-16 ***
## cos.term     0.28339    0.03813   7.432 1.07e-13 ***
## phi          0.00000         NA      NA       NA
## tau2         0.06779    0.01846   3.673 0.00024 ***
## ---
## Signif. codes:  0 `***' 0.001 `**' 0.01 `*' 0.05 `.' 0.1 ` ' 1
##
## Log pairwise likelihood: -1044.4,  CLIC: 2121.6
```

Comparison with the model without the latent process ($\tau^2 = 0$, $\phi = 0$):

```
## refit the model fixing phi = 0
pfit10.gr.nosigma <- update(pfit10.gr, fixed = c(NA, NA, NA, NA, NA, 0.0))
summary(pfit10.gr.nosigma)

##
## Call:
## lacm(formula = cases ~ trend + sin.term + cos.term,
##     data = meningo.gr, fixed = c(NA,NA, NA, NA, NA, 0), d = 1,
##     kernel.type = "Trapezoidal", gh.num = 10)
##
## Pairwise likelihood order: 1
##
## Coefficients:
##             Estimate Std. Error z value Pr(>|z|)
## (Intercept)  2.85316    0.04126   69.16   <2e-16 ***
## trend       -1.74361    0.10206  -17.08   <2e-16 ***
## sin.term     0.46886    0.02133   21.98   <2e-16 ***
```

```
## cos.term      0.27500    0.02199   12.51   <2e-16 ***
## phi           0.00000         NA      NA       NA
## tau2          0.00000         NA      NA       NA
## ---
## Signif. codes:  0  `***'  0.001  `**'  0.01  `*'  0.05  `.'  0.1  ` '  1
##
## Log pairwise likelihood: -1075.9,  CLIC: 2176.1
```

Comparison of the models based on the CLIC statistic:

```
CLIC(pfit10.gr)

## [1] 2117.39

CLIC(pfit10.gr.nophi)

## [1] 2121.606

CLIC(pfit10.gr.nosigma)

## [1] 2176.302
```

CLIC indicates that the latent autoregressive model gives a better fit than the two reduced models.

### Invasive Meningitis in Italy

Read the invasive meningitis Italian data:

```
meningo.it <- read.csv("ECDC_meningo_it.csv")
```

Visualize the series:

```
plot(ts(meningo.it$cases, start = c(1999, 1), freq = 12), ylab = "Cases", xlab ="")
```

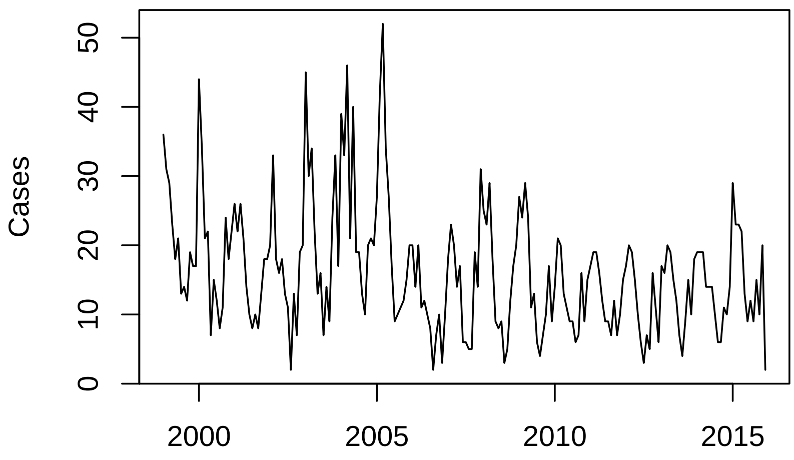

Build seasonality terms and the binary indicator that distinguishes between observations before and after March 2005:

```
meningo.it$sin.term <- sin(2 * pi * meningo.it$time / 12)
meningo.it$cos.term <- cos(2 * pi * meningo.it$time / 12)
meningo.it$trend <- meningo.it$time / nrow(meningo.it)
meningo.it$changep <- I(meningo.it$trend <= 75 / nrow(meningo.it))
```

Fit a standard Poisson regression model and obtain the Pearson residuals:

```
mod0.it <- glm(cases ~ changep + sin.term + cos.term, data = meningo.it,
        family = poisson)
res0.it <- residuals(mod0.it,  type = "pearson")
```

Plot the sample partial autocorrelation function of the Pearson residuals to select the order $d$ of the pairwise likelihood:

```
pacf(res0.it, main =" ")
```

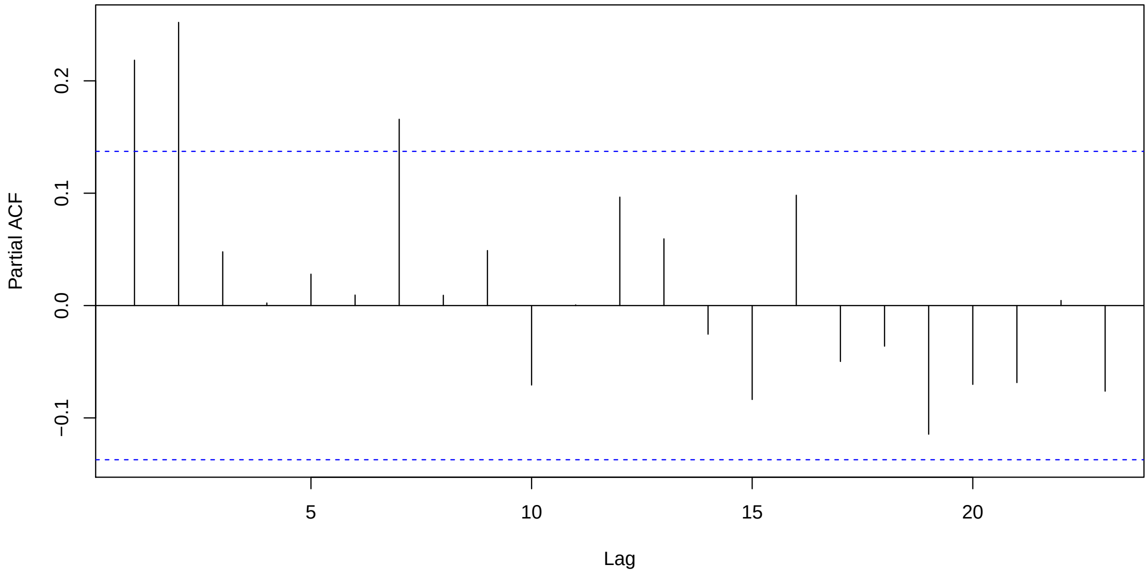


The sample partial autocorrelation suggests the presence of non-spurious correlation at the first two lags. We start with a preliminary fit of the autoregressive count model using option `fit = FALSE` in `lacm`:

```
fit.it.start <- lacm(cases ~ changep + sin.term + cos.term, data = meningo.it,
d = 2, fit = FALSE)
```

Below we calculate preliminary estimates of the dispersion indices which indicate that a low number of quadrature nodes is sufficient for approximation of the bivariate integrals of the pairwise likelihood:

```
## preliminary estimation of dispersion indices
tau2 <- fit.it.start$start.theta[6]
eta <- fit.it.start$X %*% fit.it.start$start.theta[1:4]
Di <- exp(eta + tau2 / 2) * (exp(tau2) - 1)
summary(Di)

##        V1
## Min.   :0.3782
## 1st Qu.:0.4977
## Median :0.7332
## Mean   :0.8135
## 3rd Qu.:1.0269
## Max.   :1.6169
```

Accordingly, we fit the latent autoregressive count model with the pairwise likelihood of order two with trapezoidal weights approximated with Gauss-Hermite quadrature using five nodes per dimension:

```
## load the lacm library
library(lacm)
pfit5.it <- lacm(cases ~ changep + sin.term + cos.term, data = meningo.it,
         d = 2, kernel.type = "Trapezoidal", gh.num = 5)
print(summary(pfit5.it), digits = 2)

##
## Call:
## lacm(formula = cases ~ changep + sin.term + cos.term, data = meningo.it,
##      d = 2, kernel.type = "Trapezoidal", gh.num = 5)
##
## Pairwise likelihood order: 2
##
## Coefficients:
##             Estimate Std. Error z value Pr(>|z|)
## (Intercept)    2.538      0.044    58.0   <2e-16 ***
## changepTRUE    0.376      0.072     5.3    1e-07 ***
## sin.term       0.465      0.032    14.4   <2e-16 ***
## cos.term       0.262      0.039     6.7    2e-11 ***
## phi            0.692      0.083     8.4   <2e-16 ***
## tau2           0.044      0.011     3.9    9e-05 ***
## ---
## Signif. codes:  0 `***' 0.001 `**' 0.01 `*' 0.05 `.' 0.1 ` ' 1
##
## Log pairwise likelihood: -1195.6,  CLIC: 2423
```

Refit the model with ten quadrature nodes per dimension:

```
pfit10.it <- lacm(cases ~ changep + sin.term + cos.term,data = meningo.it,
        d = 2, kernel.type = "Trapezoidal", gh.num = 10)
```

```r
print(summary(pfit10.it), digits = 2)

##
## Call:
## lacm(formula = cases ~ changep + sin.term + cos.term,  data = meningo.it,
##    d = 2, kernel.type = "Trapezoidal", gh.num = 10)
##
## Pairwise likelihood order: 2
##
## Coefficients:
##              Estimate Std. Error z value Pr(>|z|)
## (Intercept)    2.539      0.044    58.3   <2e-16 ***
## changepTRUE    0.376      0.072     5.3    1e-07 ***
## sin.term       0.466      0.032    14.6   <2e-16 ***
## cos.term       0.261      0.039     6.7    2e-11 ***
## phi            0.702      0.080     8.8   <2e-16 ***
## tau2           0.044      0.011     4.0    6e-05 ***
## ---
## Signif. codes:  0  `***'  0.001  `**'  0.01  `*'  0.05  `.'  0.1  ` '  1
##
## Log pairwise likelihood: -1195.6,  CLIC: 2423
```

Finally, with twenty quadrature nodes per dimension:

```r
pfit20.it <- lacm(cases ~ changep + sin.term + cos.term, data = meningo.it,
         d = 2, kernel.type = "Trapezoidal", gh.num = 20)
print(summary(pfit20.it), digits = 2)

##
## Call:
## lacm(formula = cases ~ changep + sin.term + cos.term, data = meningo.it,
##     d = 2, kernel.type = "Trapezoidal", gh.num = 20)
##
## Pairwise likelihood order: 2
##
## Coefficients:
##              Estimate Std. Error z value Pr(>|z|)
## (Intercept)    2.539      0.044    58.3   <2e-16 ***
## changepTRUE    0.376      0.072     5.3    1e-07 ***
## sin.term       0.466      0.032    14.6   <2e-16 ***
## cos.term       0.261      0.039     6.7    2e-11 ***
## phi            0.702      0.079     8.8   <2e-16 ***
## tau2           0.044      0.011     4.0    6e-05 ***
## ---
## Signif. codes:  0  `***'  0.001  `**'  0.01  `*'  0.05  `.'  0.1  ` '  1
##
## Log pairwise likelihood: -1195.6,  CLIC: 2423
```

Gauss-Hermite quadrature with $5 \times 5$, $10 \times 10$ and $20 \times 20$ node give the same estimates and standard errors up to two decimal digits. For the rest of the analysis we base ourselves on the model with $10 \times 10$ quadrature nodes.
Comparison with the reduced model without serial correlation ($\phi = 0$):

```
## refit the model fixing phi = 0
pfit10.it.nophi <- update(pfit10.it, fixed = c(NA, NA, NA, NA, 0.0, NA))
summary(pfit10.it.nophi)

##
## Call:
## lacm(formula = cases ~ changep + sin.term + cos.term, data = meningo.it,
##     fixed = c(NA, NA, NA, NA, 0, NA), d = 2, kernel.type = "Trapezoidal",
##     gh.num = 10)
##
## Pairwise likelihood order: 2
##
## Coefficients:
##             Estimate Std. Error z value Pr(>|z|)
## (Intercept)  2.53732    0.03642  69.668  < 2e-16 ***
## changepTRUE  0.37933    0.06118   6.201 5.63e-10 ***
## sin.term     0.46740    0.02918  16.018  < 2e-16 ***
## cos.term     0.26172    0.03580   7.311 2.64e-13 ***
## phi          0.00000         NA      NA       NA
## tau2         0.04465    0.01027   4.347 1.38e-05 ***
## ---
## Signif. codes:  0 `***' 0.001 `**' 0.01 `*' 0.05 `.' 0.1 ` ' 1
##
## Log pairwise likelihood: -1199.8,  CLIC: 2430.4
```

Comparison with the model without the latent process ($\tau^2 = 0$, $\phi = 0$):

```
## refit the model fixing phi = 0
pfit10.it.nosigma <- update(pfit10.it, fixed = c(NA, NA, NA, NA, NA, 0.0))
summary(pfit10.it.nosigma)

##
## Call:
## lacm(formula = cases ~ changep + sin.term + cos.term, data = meningo.it,
##     fixed = c(NA, NA, NA, NA, NA, 0), d = 2, kernel.type = "Trapezoidal",
##     gh.num = 10)
##
## Pairwise likelihood order: 2
##
## Coefficients:
##             Estimate Std. Error z value Pr(>|z|)
## (Intercept)  2.55854    0.02313  110.62   <2e-16 ***
## changepTRUE  0.38288    0.03292   11.63   <2e-16 ***
```

```
## sin.term     0.46691    0.01555   30.03   <2e-16 ***
## cos.term     0.25825    0.01958   13.19   <2e-16 ***
## phi          0.00000         NA      NA       NA
## tau2         0.00000         NA      NA       NA
## ---
## Signif. codes:  0  `***'  0.001  `**'  0.01  `*'  0.05  `.'  0.1  ` '  1
##
## Log pairwise likelihood: -1241.8,  CLIC: 2510
```

Comparison of the models based on the CLIC statistic:

```
CLIC(pfit10.it)

## [1] 2423.077

CLIC(pfit10.it.nophi)

## [1] 2430.35

CLIC(pfit10.it.nosigma)

## [1] 2509.97
```

CLIC indicates that the latent autoregressive model gives a better fit than the two reduced models.

# 2 Simulation results

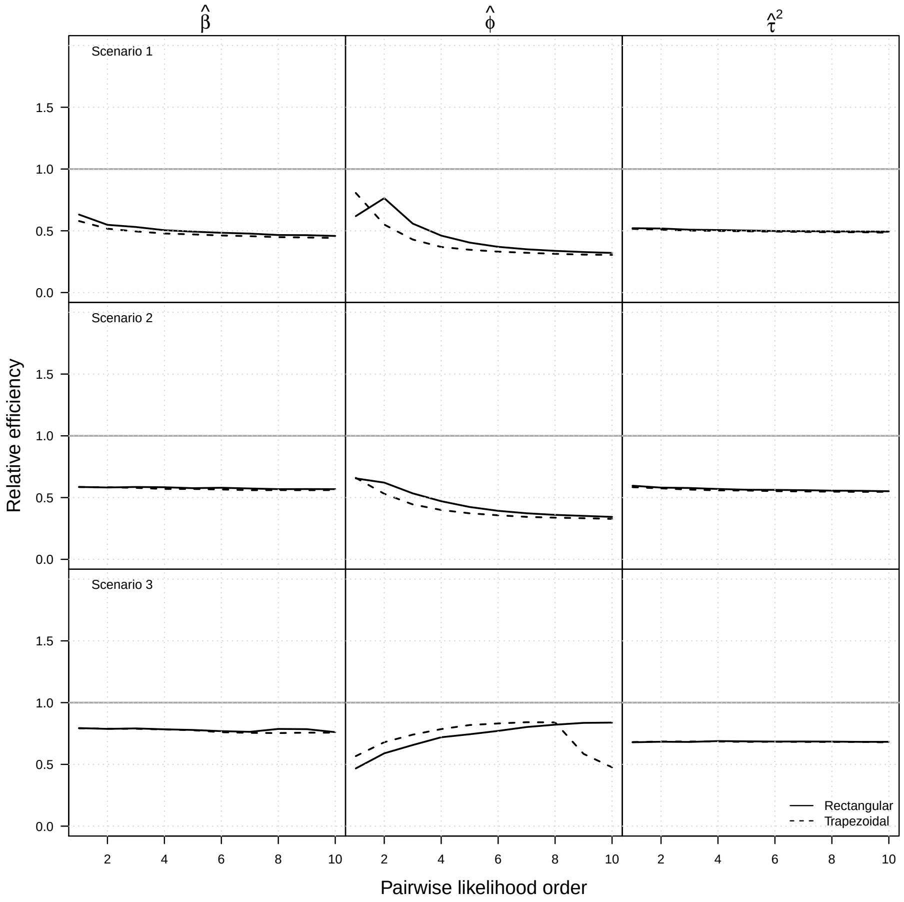


**Figure SM1:** Relative efficiency of maximum pairwise likelihood estimates with respect to INLA estimates as a function of the pairwise likelihood order $d$ for simulation scenarios 1 (upper panel), 2 (mid panel) and 3 (bottom panel). The pairwise likelihood is approximated with Gauss-Hermite quadrature with 5 quadrature nodes per dimension using rectangular or trapezoidal weights.

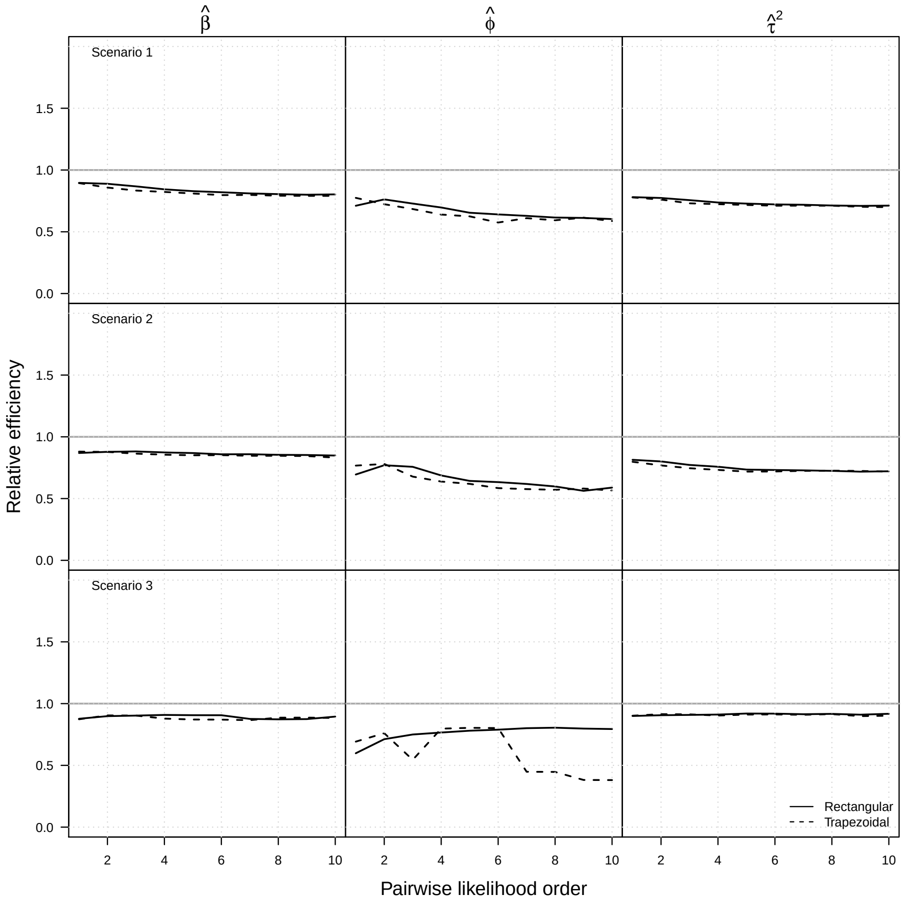


**Figure SM2:** Relative efficiency of maximum pairwise likelihood estimates with respect to INLA estimates as a function of the pairwise likelihood order $d$ for simulation scenarios 1 (upper panel), 2 (mid panel) and 3 (bottom panel). The pairwise likelihood is approximated with Gauss-Hermite quadrature with 10 quadrature nodes per dimension using rectangular or trapezoidal weights.

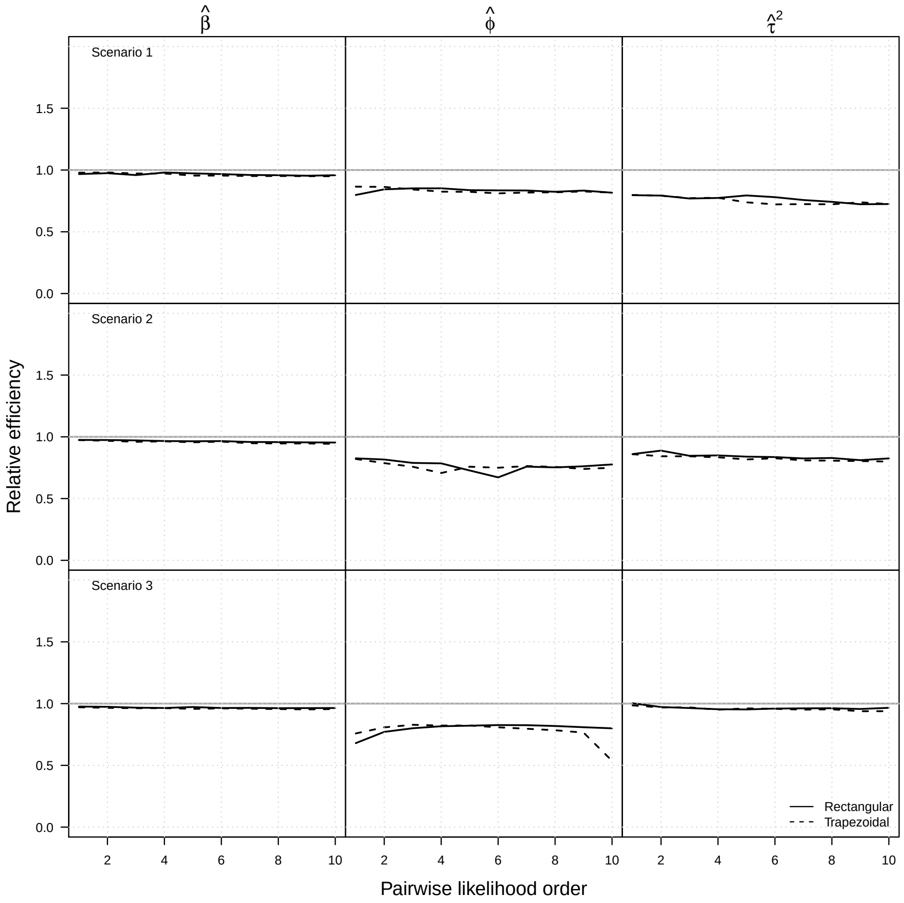


**Figure SM3:** Relative efficiency of maximum pairwise likelihood estimates with respect to INLA estimates as a function of the pairwise likelihood order $d$ for simulation scenarios 1 (upper panel), 2 (mid panel) and 3 (bottom panel). The pairwise likelihood is approximated with Gauss-Hermite quadrature with 30 quadrature nodes per dimension using rectangular or trapezoidal weights.

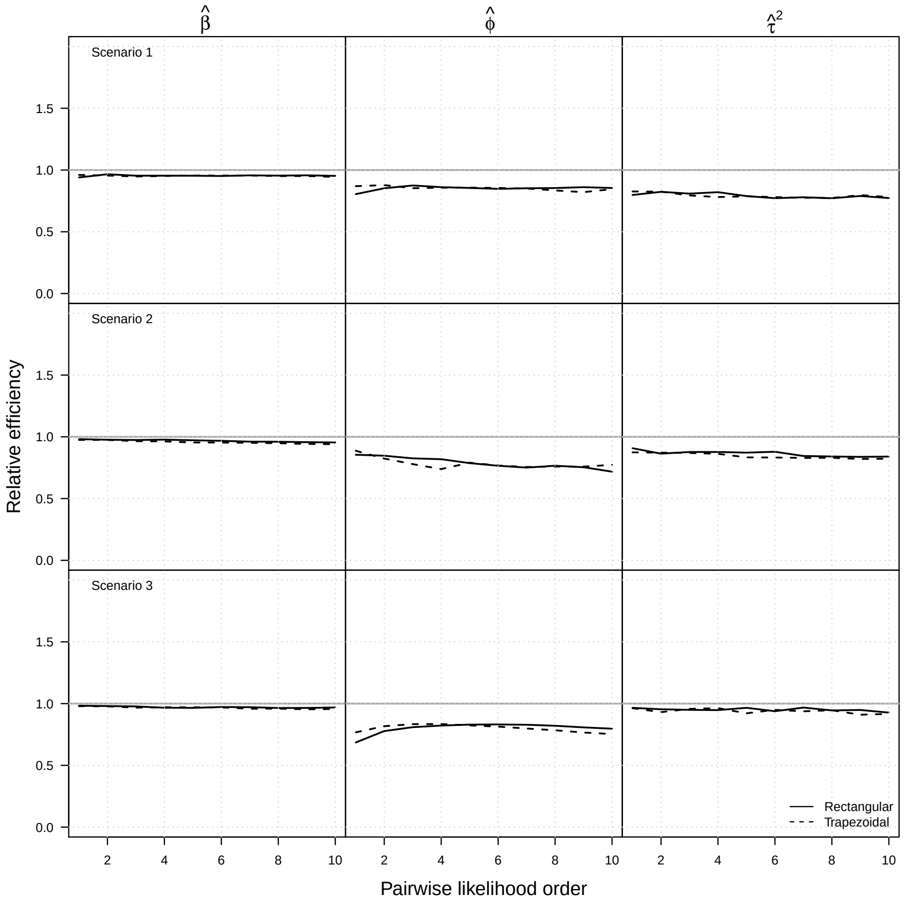


**Figure SM4:** Relative efficiency of maximum pairwise likelihood estimates with respect to INLA estimates as a function of the pairwise likelihood order $d$ for simulation scenarios 1 (upper panel), 2 (mid panel) and 3 (bottom panel). The pairwise likelihood is approximated with Gauss-Hermite quadrature with 40 quadrature nodes per dimension using rectangular or trapezoidal weights.
